# Supplementary material for: How to Overcome Curse-of-Dimensionality for Out-of-Distribution Detection?
Source: arXiv:2312.14452 source file (2023-12-22)
Supplement: Supplementary file 1 [file appendix.tex]

\appendix

\section{Societal Impact}

\section{Proof of Theorem 4.1}
\label{sec:proof_sup}
Recall that  local density estimation can be performed by $k$-NN distance~\cite{sun2022knn}: 
\begin{equation*}
\label{eq:estimate}
    \hat{p}(\*z) = c_{k, N} r_k\left(\mathbf{z}\right)^{1-m},
\end{equation*} where $c_{k, N}$ is a constant value dependent on the $k$ and training set size $N$ and $\*z$ is the normalized feature embedding for $\*x$. Our goal is to prove the following Theorem 4.1:

\begin{theorem} (Recap of Theorem 4.1) 
    Denote normalized feature vectors for ID and OOD samples as $\*z_{in}$, $\*z_{out}$. 
     Let the gap in the $k$-NN distance be $\delta_r = r_k\left(\mathbf{z}_{out}\right) -r_k\left(\mathbf{z}_{in}\right)$, the following equation holds with proof: 
     \begin{equation*}
         \delta_r = r_k(\mathbf{z}_{in}) [(1 - \frac{\delta_p}{c_{k, N}} r_k(\mathbf{z}_{in})^{m-1})^{-\frac{1}{m-1}} - 1]
     \end{equation*}
\end{theorem}

\textit{Proof:}
\begin{align*}
\small
\delta_r &= r_k\left(\mathbf{z}_{out}\right) -r_k\left(\mathbf{z}_{in}\right) \\
&= (r_k\left(\mathbf{z}_{out}\right)^{1-m})^{-\frac{1}{m-1}} -r_k\left(\mathbf{z}_{in}\right) \\
    &= (r_k\left(\mathbf{z}_{in}\right)^{1-m} - (r_k\left(\mathbf{z}_{in}\right)^{1-m} - r_k\left(\mathbf{z}_{out}\right)^{1-m}))^{-\frac{1}{m-1}}  -r_k\left(\mathbf{z}_{in}\right) \\
    &= (r_k\left(\mathbf{z}_{in}\right)^{1-m} - \frac{\delta_p}{c_{k, N}} )^{-\frac{1}{m-1}}  -r_k\left(\mathbf{z}_{in}\right) \\
    &= r_k(\mathbf{z}_{in}) [(1 - \frac{\delta_p}{c_{k, N}} r_k(\mathbf{z}_{in})^{m-1})^{-\frac{1}{m-1}} - 1].  \quad \quad \quad \square
\end{align*}

\section{Training Details}
\label{app:train}

\section{Validation Strategy}
\label{app:validation}

\section{SNN compatible with parametric approaches}

\newcolumntype{?}{!{\vrule width 1pt}}
\begin{table}[h]
\centering
\resizebox{0.95\columnwidth}{!}{%
\begin{tabular}{lccc}
\textbf{Method} & \textbf{Dataset (ID)} & \textbf{FPR95}  & \textbf{AUROC} \\
& & \downarrow & \uparrow  \\
\toprule
Mahalanobis~\cite{lee2018simple} & CIFAR-10 & 40.58 & 84.81  \\
\rowcolor{COLOR_ZS} \name (w. Mahalanobis) & CIFAR-10 &  \textbf{30.95} &  \textbf{89.72} \\
\midrule
Mahalanobis~\cite{lee2018simple} & CIFAR-100 & 56.27 & 78.54  \\
\rowcolor{COLOR_ZS} \name (w. Mahalanobis) & CIFAR-100 &  \textbf{53.96} &  \textbf{80.22} \\
\bottomrule
\end{tabular}}
\caption{\name is also compatible with parametric approaches such as Mahalanobis distance~\cite{lee2018simple}. All values are averaged over multiple OOD test datasets.}
\label{tab:compatibility}
\end{table}

\section{Description of OOD baselines}
\label{app:ood_description}
In this section, we include a brief description of all the compared OOD baseline methods.

\paragraph{Maximum Softmax Probability (MSP) \cite{hendrycks2016baseline}} uses the maximum value corresponding to softmax probability vector as confidence scores to detect OOD examples.

\paragraph{ODIN \cite{liang2018enhancing}} ODIN utilizes the calibrated confidence scores computed using temperature scaling and input perturbations for OOD detection. Perturbation Magnitude $\eta$ is chosen by validating on 1000 images randomly sampled from in-distribution test set. We set temperature parameter ($T$) = 1000 for all experiments on CIFAR-10/100 benchmark. Specifically, for DenseNet-101, we set $\eta$ = 0.0016 for CIFAR-10 and $\eta$ = 0.0012 for CIFAR-100.

\paragraph{Mahalanobis \cite{lee2018simple}} uses Mahalanobis distance-based confidence scores for OOD detection. 

% For fine-tuning the perturbation magnitude $\eta$, we train a Logistic Regression model using 1000 randomly sampled examples from ID test set ($\mathcal{D}^{test}_{in}$) and adversarial examples generated by applying FGSM~\cite{goodfellow2014explaining} on them with a perturbation of size 0.05. $\eta$ is chosen from \{0.0, 0.01, 0.005, 0.002, 0.0014, 0.001, 0.0005\} such that it optimizes the TNR@TPR95.

\paragraph{Generalized-ODIN \cite{hsu2020generalized}} Hsu \etal propose a decomposed confidence model for the purpose of \ood detection, where the logits($f$) of a classifier is  defined using a dividend/divisor structure as follows: $	f(x) =\frac{h(x)}{g(x)}$, where $h(x)$ and $g(x)$ are two functions. The authors propose three variants of \ood detectors, namely, DeConf-I, DeConf-E and DeConf-C which uses Inner-Product, Negative Euclidean Distance and Cosine Similarity for defining $h(x)$ respectively. In this study, we use the DeConf-C variant, since it is shown to be the most robust of all the variants. For calculating \ood score we use the output of $h(x)$ function.

\paragraph{LogitNorm~\cite{wei2022mitigating}}
\paragraph{DICE~\cite{sun2022dice}}

\paragraph{KNN~\cite{sun2022knn}}

\section{Software and Hardware}
\label{app:hardware}
We run all experiments with Python 3.7.4 and PyTorch 1.9.0. For experiments on CIFAR-10/100 benchmarks, we use Nvidia RTX 2080-Ti GPUs. Experiments on ImageNet-100 are run on Nvidia Tesla A100 GPU.

\section{Extension: Post-hoc Calibration results}
\label{app:post_hoc_calib}

\section{Extension: Detailed Results}
\label{app:results}

\section{Proof of Main Theorem}
\label{app:proof}
